# Supplementary material for: AppealNet: An Efficient and Highly-Accurate Edge/Cloud Collaborative Architecture for DNN Inference
Source: arXiv:2105.04104 source file (2021-11-25)
Supplement: Supplementary file 1 [file appendix.tex]

\appendix

\section{Probability Interpretation of AppealNet}
\label{appendix:prob}
We explain the objective function derived in Section~\ref{subsec:bba} from the probabilistic aspect and cast our formulation as learning probability distributions in this section. 

For better illustration, we abbreviate $q(1|\mathbf{x})$ and $f_1(\mathbf{x})$ as $z$ and $y_f$ respectively, and rewrite Eq.~\eqref{eq:final-re-m} as Eq.~\eqref{eq:prob-1}.
\begin{equation}
	z \cdot \ell (y_f,y) + \beta (-log(z))
	\label{eq:prob-1}
\end{equation}

Considering $\ell (y_f,y)$ is a positive constant, the above equation becomes a function of $z$. Assuming $\bar{z}$ as a \textit{critical point} of the objective function, then we have:
\begin{equation}
	\ell (y_f,y) = \beta \frac{1}{z}
	\label{eq:prob-2}
\end{equation}

We emphasize that both loss $\ell (y_f,y)$ and the derivation of $log(z)$ (\textit{i.e.}, $\frac{1}{z}$) are positive, which guarantees the critical point $\bar{z}$ always exists. Eq.~\eqref{eq:prob-2} implies that the predictor $z=q(1|\mathbf{x})$ provides the expectation loss of the little network for a given input $\mathbf{x}$:
\begin{equation}
	\mathbb{E} [\ell (f_1(\mathbf{x}), y)] = \beta \frac{1}{z}
	\label{eq:prob-3}
\end{equation}

Considering a common regression task, where $y$ is continuous scalar and $\ell$ is $L2$ loss (classification tasks can be analyzed in a similar approach):
\begin{equation}
	\ell (y_f, y) = (y_f-y)^2
	\label{eq:prob-4}
\end{equation}

Based on the Eq.~\eqref{eq:prob-3} and~\eqref{eq:prob-4}, we estimate that:

\begin{equation}
	y_f = \text{arg} \min_{\mu} \mathbb{E}_{P(y|\mathbf{x})}[(y-\mu)^2]=\mathbb{E}_{P(y|\mathbf{x})}[y] 
\end{equation}
\begin{equation}
	\beta \frac{1}{z} = \mathbb{E}_{P(y|\mathbf{x})}[(y-\mu)^2] = \text{Var}_{P(y|\mathbf{x})}[y]
\end{equation}

As a result, the optimization objective arrived in Eq.~\eqref{eq:final-re-m} learns a Gaussian distribution $\mathcal{N}(y|\mu(\mathbf{x}),\sigma^2(\mathbf{x}))$, wherein $y_f=f_1(\mathbf{x})$ fits the expectation of $y$ and $z=q(1|\mathbf{x})$ yields the variance of $y$:
\begin{equation}
	P(y|\mathbf{x}, \mu, \sigma) = \frac{1}{\sqrt{2\pi}\sigma}e^{-(y-\mu)^2/2\sigma^2}, \mu = y_f, \sigma^2 = \frac{\beta}{z}
\end{equation}

In this case, the larger the predictor output $q(1|\mathbf{x})$ is, the smaller the variance of $y$ estimated, hence the more confident the little network is with respect to $\mathbf{x}$. 
Therefore, the confidence estimated by the predictor can act as an trustworthy indicator of whether the input can be processed by the little network or not.

\section{AppealNet Training Details}
\label{appendix:setup}

\subsection{Loss Function of AppealNet}
\label{appendix:loss}
% for both classification and regression. 
We elaborate the loss function for AppealNet in this section.
Let $p_z$ be the abbreviation of prediction and $q$ be the output of the predictor. For $K$-class classification tasks, $p_z$ is the predictive probability vector in $K$-dimension ($p_{zi} \in (0, 1)$). 
% For regression, $p_z$ is a continues scalar. Moreover, $q$ is in the range of $(0, 1)$ for both cases.

% \begin{enumerate}
% 	\item
% 	\textit{Classification Tasks}. 
With the above, the following Eq. \eqref{ls-1} denotes the loss function for the approximator. %in classification tasks. 
Note that, under black-box setting stated in Section~\ref{subsec:bba}, we can simply replace $p_{0i}$ as $y_i$ and keep the remaining terms unchanged.
\begin{equation}
\mathcal{L}_p = q\cdot \sum_{i=1}^{K}-log(p_{1i}) \cdot y_i + 
(1-q) \cdot \sum_{i=1}^{K}-log(p_{0i}) \cdot y_i
\label{ls-1}
\end{equation}
% \begin{equation}
% 	\mathcal{L}_p = \sum_{i=1}^{K}-log[(q \cdot p_{1i} + (1 - q) \cdot p_{0i})]\cdot y_i
% 	\label{ls-2}
% \end{equation}

% Similarly, we can draw the counterpart \eqref{ls-3} for regression tasks. Here we consider $L2$ loss, but the formulation could generalize to other regression losses. 
% \begin{equation}
% \mathcal{L}_p = q \cdot |p_1 - y|^2 + (1-q) \cdot |p_0 - y|^2
% \label{ls-3}
% \end{equation}

% 	\begin{equation}
% 	\mathcal{L}_p = |q\cdot p_1 + (1-q)\cdot p_0 - y |^2
% 	\label{ls-4}
% 	\end{equation}
% \end{enumerate}

The loss function for the predictor is illustrated in Eq. \eqref{ls-5}, wherein the target of optimization is to minimize the log-likelihood of $q$. 
\begin{equation}
\mathcal{L}_q = -log(q)
\label{ls-5}
\end{equation}

Finally, we arrive at the total loss, which is simply a weighted sum of $\mathcal{L}_p$ and $\mathcal{L}_q$ with a hyperparameter $\beta$:
\begin{equation}
\mathcal{L}_{total} = \mathcal{L}_p + \beta \cdot \mathcal{L}_q
\label{ls-6}
\end{equation}

% The computation flow of forwarding the input to B/L system and calculating the loss is illustrated in Figure~\ref{fig:cb-loss}. 
%Here we go deeper into the dynamics of proposed loss function as follow. 
When optimizing $\mathcal{L}_p$, the gradient for $q$ (always negative) pushes it towards $0$, while the gradient from $\mathcal{L}_q$ (always positive) pushes it towards $1$. Such kind of adversarial objectives facilitates to differentiate those "easy" inputs and "difficult" inputs during training, as can be seen with the visualization of $q(z|\textbf{x})$ in Section~\ref{subsec:vo} and Appendix~\ref{appendix:input}.

\subsection{Dynamic Adjustment of Lagrangian Multiplier $\beta$}
\label{appedix:beta}
The hyper-parameter $\beta$ controls the relative importance of cost constraint to the total objective.  From our experiments, we find out that searching $\beta$ on the validation dataset and fix $\beta$ during training cannot always find satisfactory results. It sometimes leads to outputting unity prediction from the predictor (\textit{i.e.}, $q(1|\mathbf{x})\rightarrow 1$). We monitor the learning curve of the predictor loss $\mathcal{L}_q$ and observe the over-fitting of predictor $q$. %Thus, some regularization methods are in need. 

\begin{figure*}[t]
	\centering
	\includegraphics[width=0.85\linewidth]{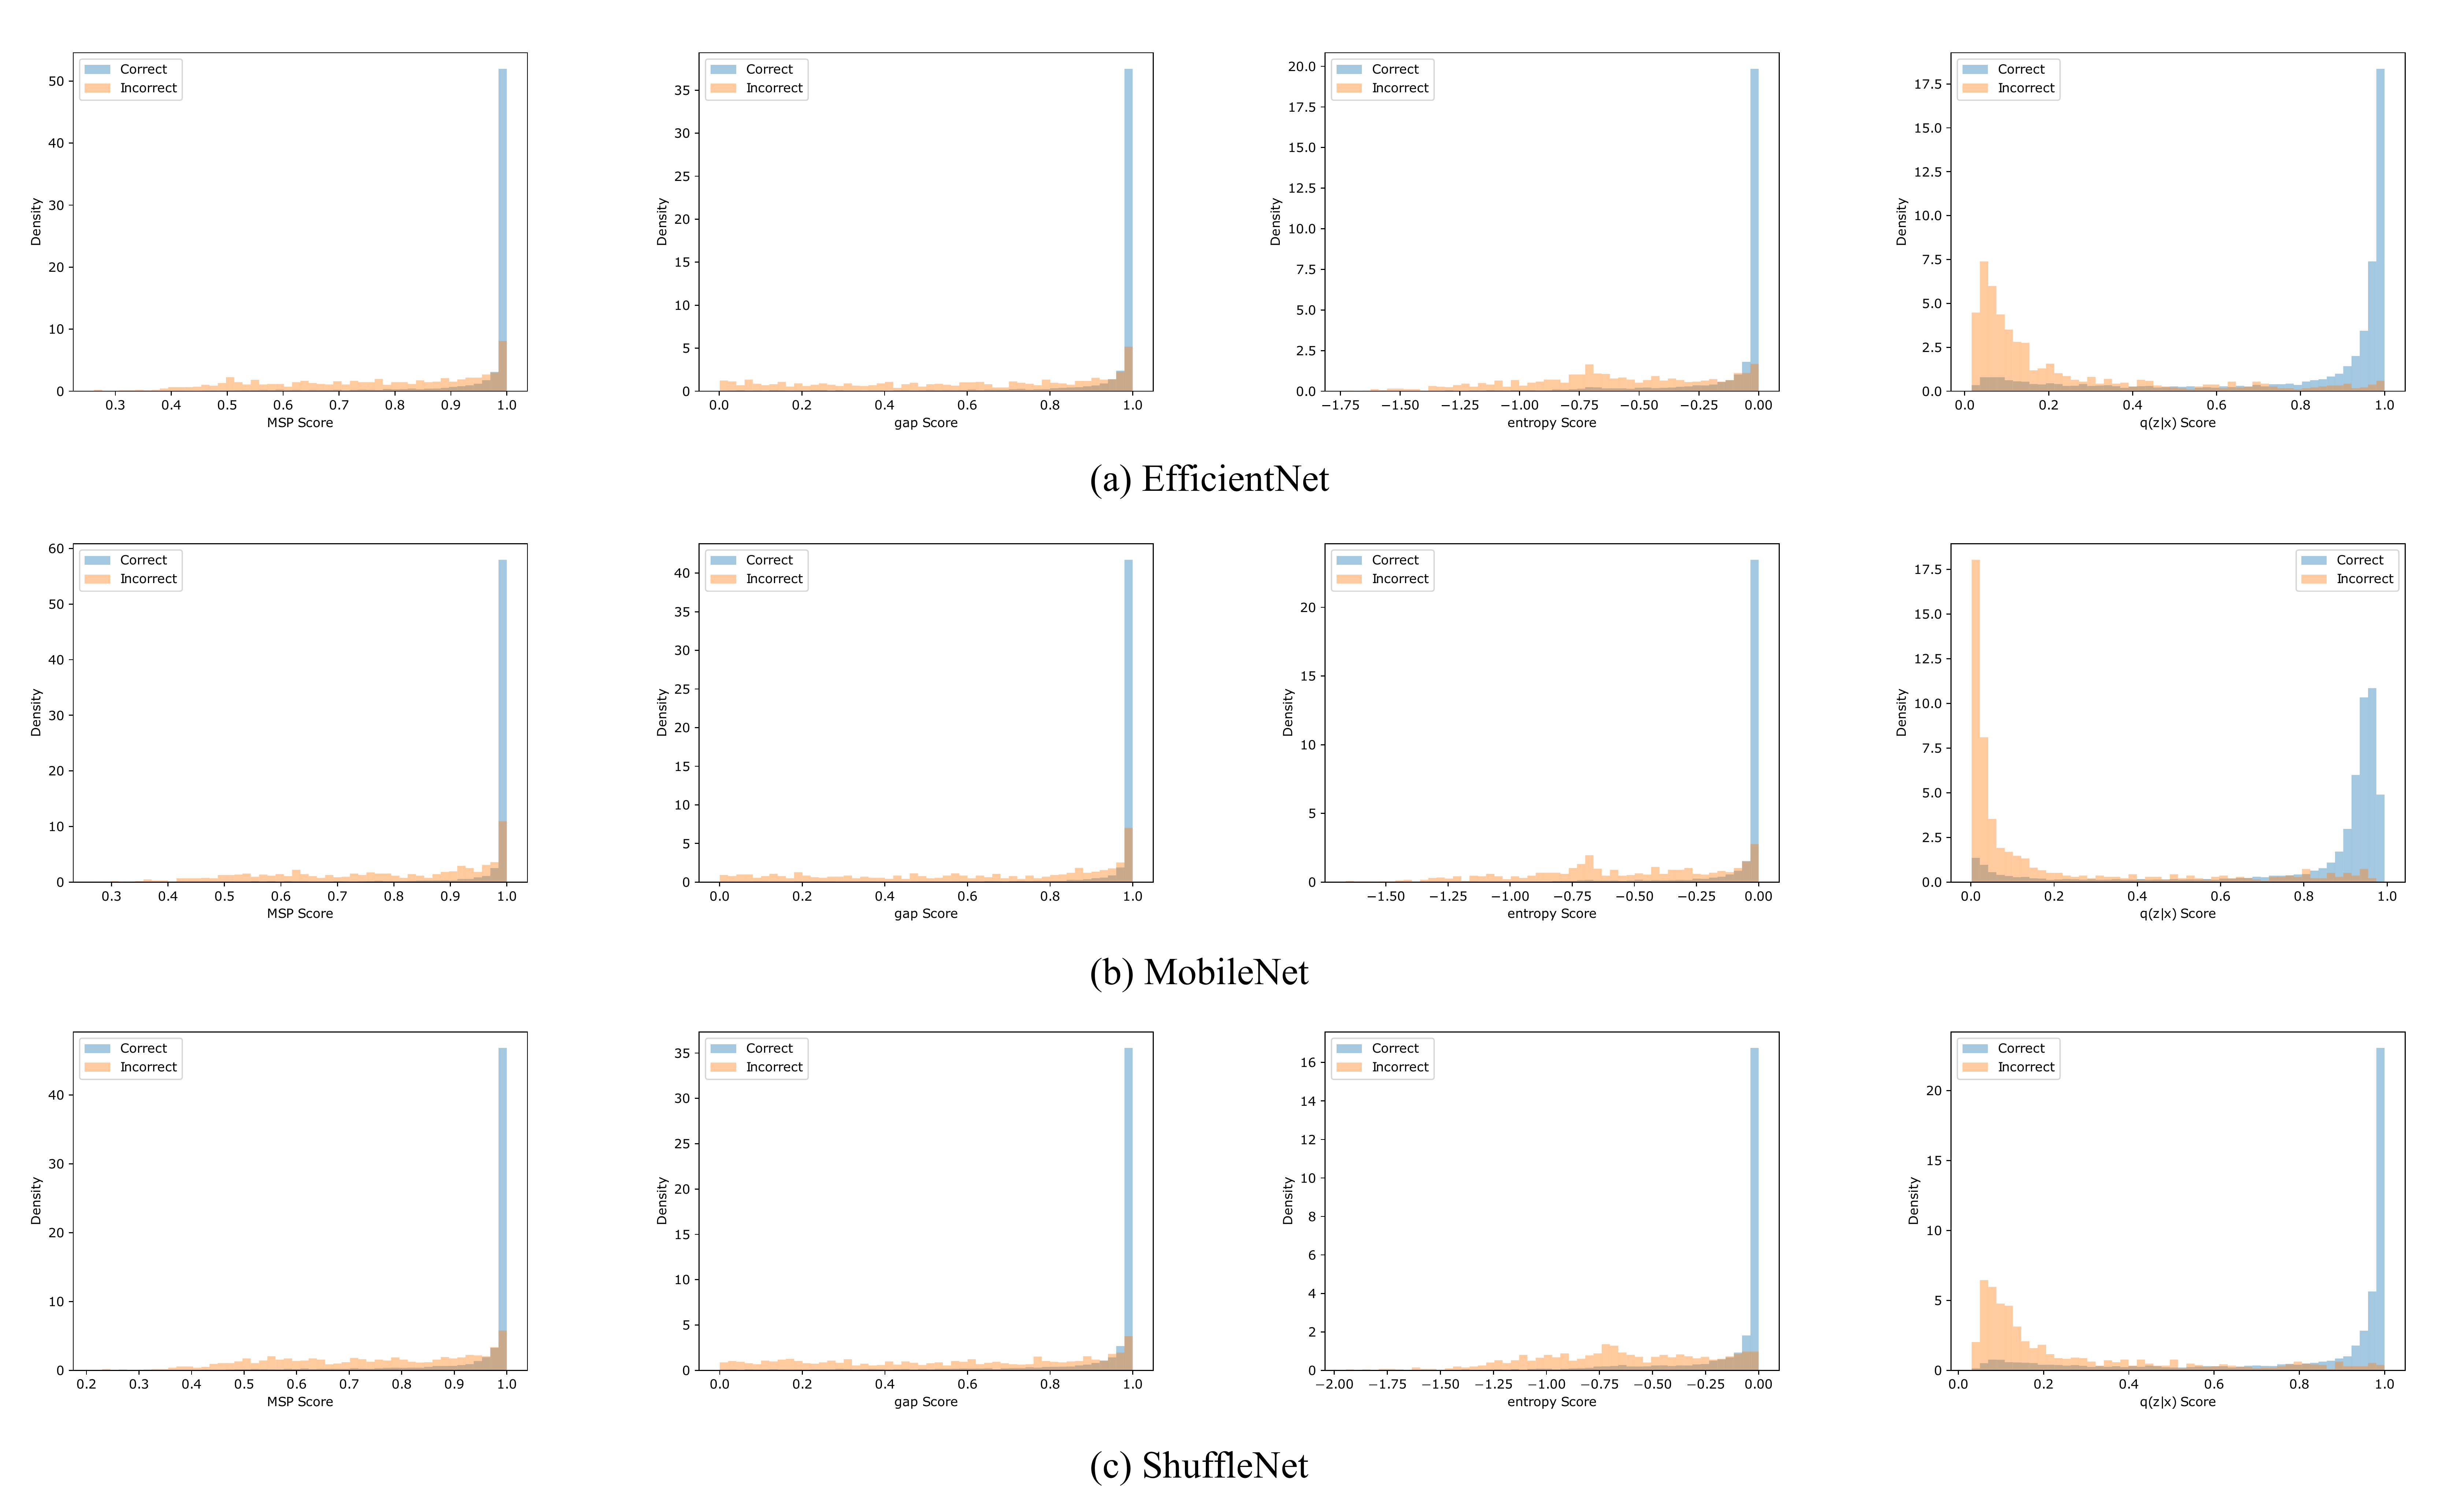}
	\caption{Histogram of three baseline solutions and AppealNet on CIFAR-10.}
	\label{fig:four-conf}
\end{figure*}

We then adopt the dynamic adjustment strategy proposed in ~\cite{devries2018learning} to resolve the above issue. The complete algorithm of joint training is illustrated in Algorithm~\ref{algo:jt-complete}, where the dynamic adjustment strategy of $\beta$ is from line 7 to line 10. To be specific, we introduce an auxiliary input named \textit{expected predictor loss} $\alpha$. During training, we not only update the model weights by descending stochastic gradients (line 4 to line 6), but also adjust the Lagrange multiplier $\beta$ such that the loss of predictor $\mathcal{L}_q$ converge to $\alpha$ (line 7 to line 10): if $\mathcal{L}_q > \alpha$, we then increase $\beta$ by a small step, and vice versa. We set $\alpha$ as 0.5 for all datasets in our experiments.

\begin{algorithm}[t]
	\caption{Complete Joint Training for Two-Head Little Network.}
	\label{algo:jt-complete}
	\KwIn{ Dataset $\textbf{S}$ sampled from $P(\textbf{x},y)$, 
		Big Network $f_0$, Expected predictor loss $\alpha$.}
	\KwOut{Little Network $(f_1, q)$.}
	\tcc{Initialize}
	 Initialize $f_1$ with the pre-trained model\;
	 Insert the predictor head and get two-head little network $(f_1, q)$\;
	%$\beta \gets 0.1$\;
	\tcc{Training Process}
	\While{Not Convergence}{
		Sample ${(\textbf{x}_1, y_1),\cdots,(\textbf{x}_M, y_M)}$ from $\textbf{S}$\;
		\tcc{$\mathcal{L}_q$ and $\mathcal{L}_p$ depend on tasks and settings}
		$\mathcal{L} = \frac{1}{M}\sum_{i}[\mathcal{L}_p(\textbf{x}_i, y_i|f_0,f_1,q)+
		\beta \mathcal{L}_q(\textbf{x}_i|q)]$\;
		Update $(f_1, q)$ by descending stochastic gradient of $\mathcal{L}$ \;
				\tcc{Dynamic Adjustment of $\beta$}
				\eIf{$\frac{1}{M}\sum_{i=1}^{M}\mathcal{L}_q^i(\textbf{x}_i, y_i) > \alpha$}
				{	
					$\beta \gets (\beta \setminus 0.99)$ \tcp*{Increase $\beta$}
				} 
				{	
					$\beta \gets (\beta \setminus 1.01)$ \tcp*{Decrease $\beta$}
				}
	}
	
	\Return Little Network$(f_1, q)$;
\end{algorithm}

\subsection{Datasets}
\label{appendix:dataset}
We demonstrate the effectiveness of AppealNet using four classification datasets: The German Traffic Sign Recognition Benchmark (GTSRB)~\cite{stallkamp2012man}, CIFAR-10, CIFAR-100~\cite{krizhevsky2009learning}, Tiny-ImageNet~\cite{deng2009imagenet}. 
GTSRB collects different traffic signs with 43 classes, containing 39,209 training images and 12,630 test images with various image sizes. We resize them to 32x32 pixels for evaluation. The two CIFAR {data-sets} both consist of 60,000 (50,000 for training and 10,000 for testing) 32x32 color images of 10 and 100 classes, respectively. 
Tiny-ImageNet is a 200-class natural image dataset sub-sampled from ImageNet dataset and it contains 100,000 training and 10,000 testing images.

\subsection{Neural Network Specification}
\label{appendix:nn}
\begin{table}[t]
	\resizebox{\columnwidth}{!}{
		\begin{tabular}{c|ccc|c}
			\hline
			Cost         & MobileNet & EfficientNet & ShuffleNet & ResNet-101 \\ \hline
			MFLOPs  & 94.61     & 31.43        & 11.42      & 2520.29    \\
			M \#Params & 2.30      & 3.60         & 0.35       & 42.52      \\ \hline
	\end{tabular}}
% 	\vspace{10pt}
	\caption{Computational and storage cost of CNNs on a 10-class classification task.}
	\label{tb:cost}
\end{table}

We evaluate AppealNet design on three off-the-shelf efficient CNN models as the little network: MobileNet~\cite{howard2017mobilenets}, EfficientNet~\cite{TanL19}, and ShuffleNet~\cite{ZhangZLS18}. They can be deployed on a diverse range of mobile/IoT devices with different hardware cost. We choose ResNet-101~\cite{he2016deep} as the big network, which achieves state-of-the-art performance across three datasets. 
In particular, we use a \textit{width multiplier} of 0.5 to train all little networks for the GTSRB and follow the original implementations to train the neural networks for CIFAR-10, CIFAR-100 and Tiny-ImageNet. Except for the Tiny-ImageNet model whose input size is 224x224, all other base models accept 32x32 inputs. Table~\ref{tb:cost} lists the computational cost (FLOPs) and storage cost ($\#$ of parameters) of these neural networks, whose task is a 10-class classification. Note that the auxiliary predictor head induces negligible overhead for both computational and storage costs.

For evaluation, we take the computational cost as the major concern rather than the storage cost. This is because, during deployment, once the parameters are loaded into the memory on devices, the storage cost is fixed. %We should always select the efficient DNN whose size is under the storage constraint of specific hardware. 
However, the computational cost of B/L system is dynamic depending on the appealing strategy and the computational cost of both Big/Little networks. Also, the computational cost is a major indicator for other concerns such as latency and energy savings. Therefore, we use the overall computational cost as one of the main evaluation metrics for comparison, which is defined in Eq.~\eqref{eq:overall-cost}.

% All networks are optimized using Adam optimizer~\cite{kingma2014adam} with the weight decay of $10e^{-6}$ and mini-batch size of 128 for 300 epochs. The learning rate is initialized to $3e^{-4}$ and updated using a cosine annealing schedule~\cite{loshchilov2016sgdr} after 10$^{th}$ epochs. We also use standard data augmentation methods, including random cropping, padding, and horizontal flipping. 
% All networks are optimized using SGD optimizer~\cite{bottou2010large} with the weight decay of 5e-4 and mini-batch size of 128 for 200 epochs. The learning rate is initialized to $0.1$ and updated using a step-decay schedule at the $60^{th}$, $120^{th}$ and $160^{th}$ epochs by 0.2. We also use standard data augmentation methods, including random cropping, padding, and horizontal flipping. 

\subsection{Training methods}
% How we train the model, including the fine-tuning strategy.

All networks are optimized using SGD optimizer~\cite{bottou2010large} with the weight decay of 5e-4 and mini-batch size of 128 for 200 epochs. The learning rate is initialized as 0.1 if we train the model from scratch and 0.01 if we fine-tune a pre-trained model, and update the learning rate using a step-decay schedule at the $60^{th}$, $120^{th}$ and $160^{th}$ epochs by 0.2. We also use standard data augmentation methods, including random cropping, padding, and horizontal flipping. 

To guarantee fair comparison, in all experiments, AppealNet is initialized with the pre-trained network without predictor head and then fine-tuned on the same datasets. By doing so, the accuracy of AppealNet and other models is close enough to void the impact of model accuracy on input differentiation (See model accuracy in Table~\ref{tb:baseline}).

\section{More Experimental Results}
\label{appendix:more}
\subsection{Visualization of Input Differentiation}
\label{appendix:input}
Figure~\ref{fig:four-conf} visualizes the MSP, Gap, Entropy and $q(z|\mathbf{x})$ scores with three different neural network architectures as the little network on CIFAR-10. 
We find that the score distributions generated by three baseline solutions are similar (first three columns), and none of them can separate inputs well. However, $q(z|\mathbf{x})$ score (last column) from AppealNet is able to differentiate the "easy" inputs and "difficult" inputs well.

Besides CIFAR-10, the input differentiation of AppealNet is also effective on other datasets. To illustrate this fact, we visualize the MSP score and $q(z|\mathbf{x})$ score with MobileNet as the littler network on CIFAR-100 and Tiny-ImageNet in Figure~\ref{fig:two-conf}. 
The results of Gap scores and Entropy scores are similar to that of MSP scores.
\begin{figure}[]
	\centering
	\includegraphics[width=0.85\linewidth]{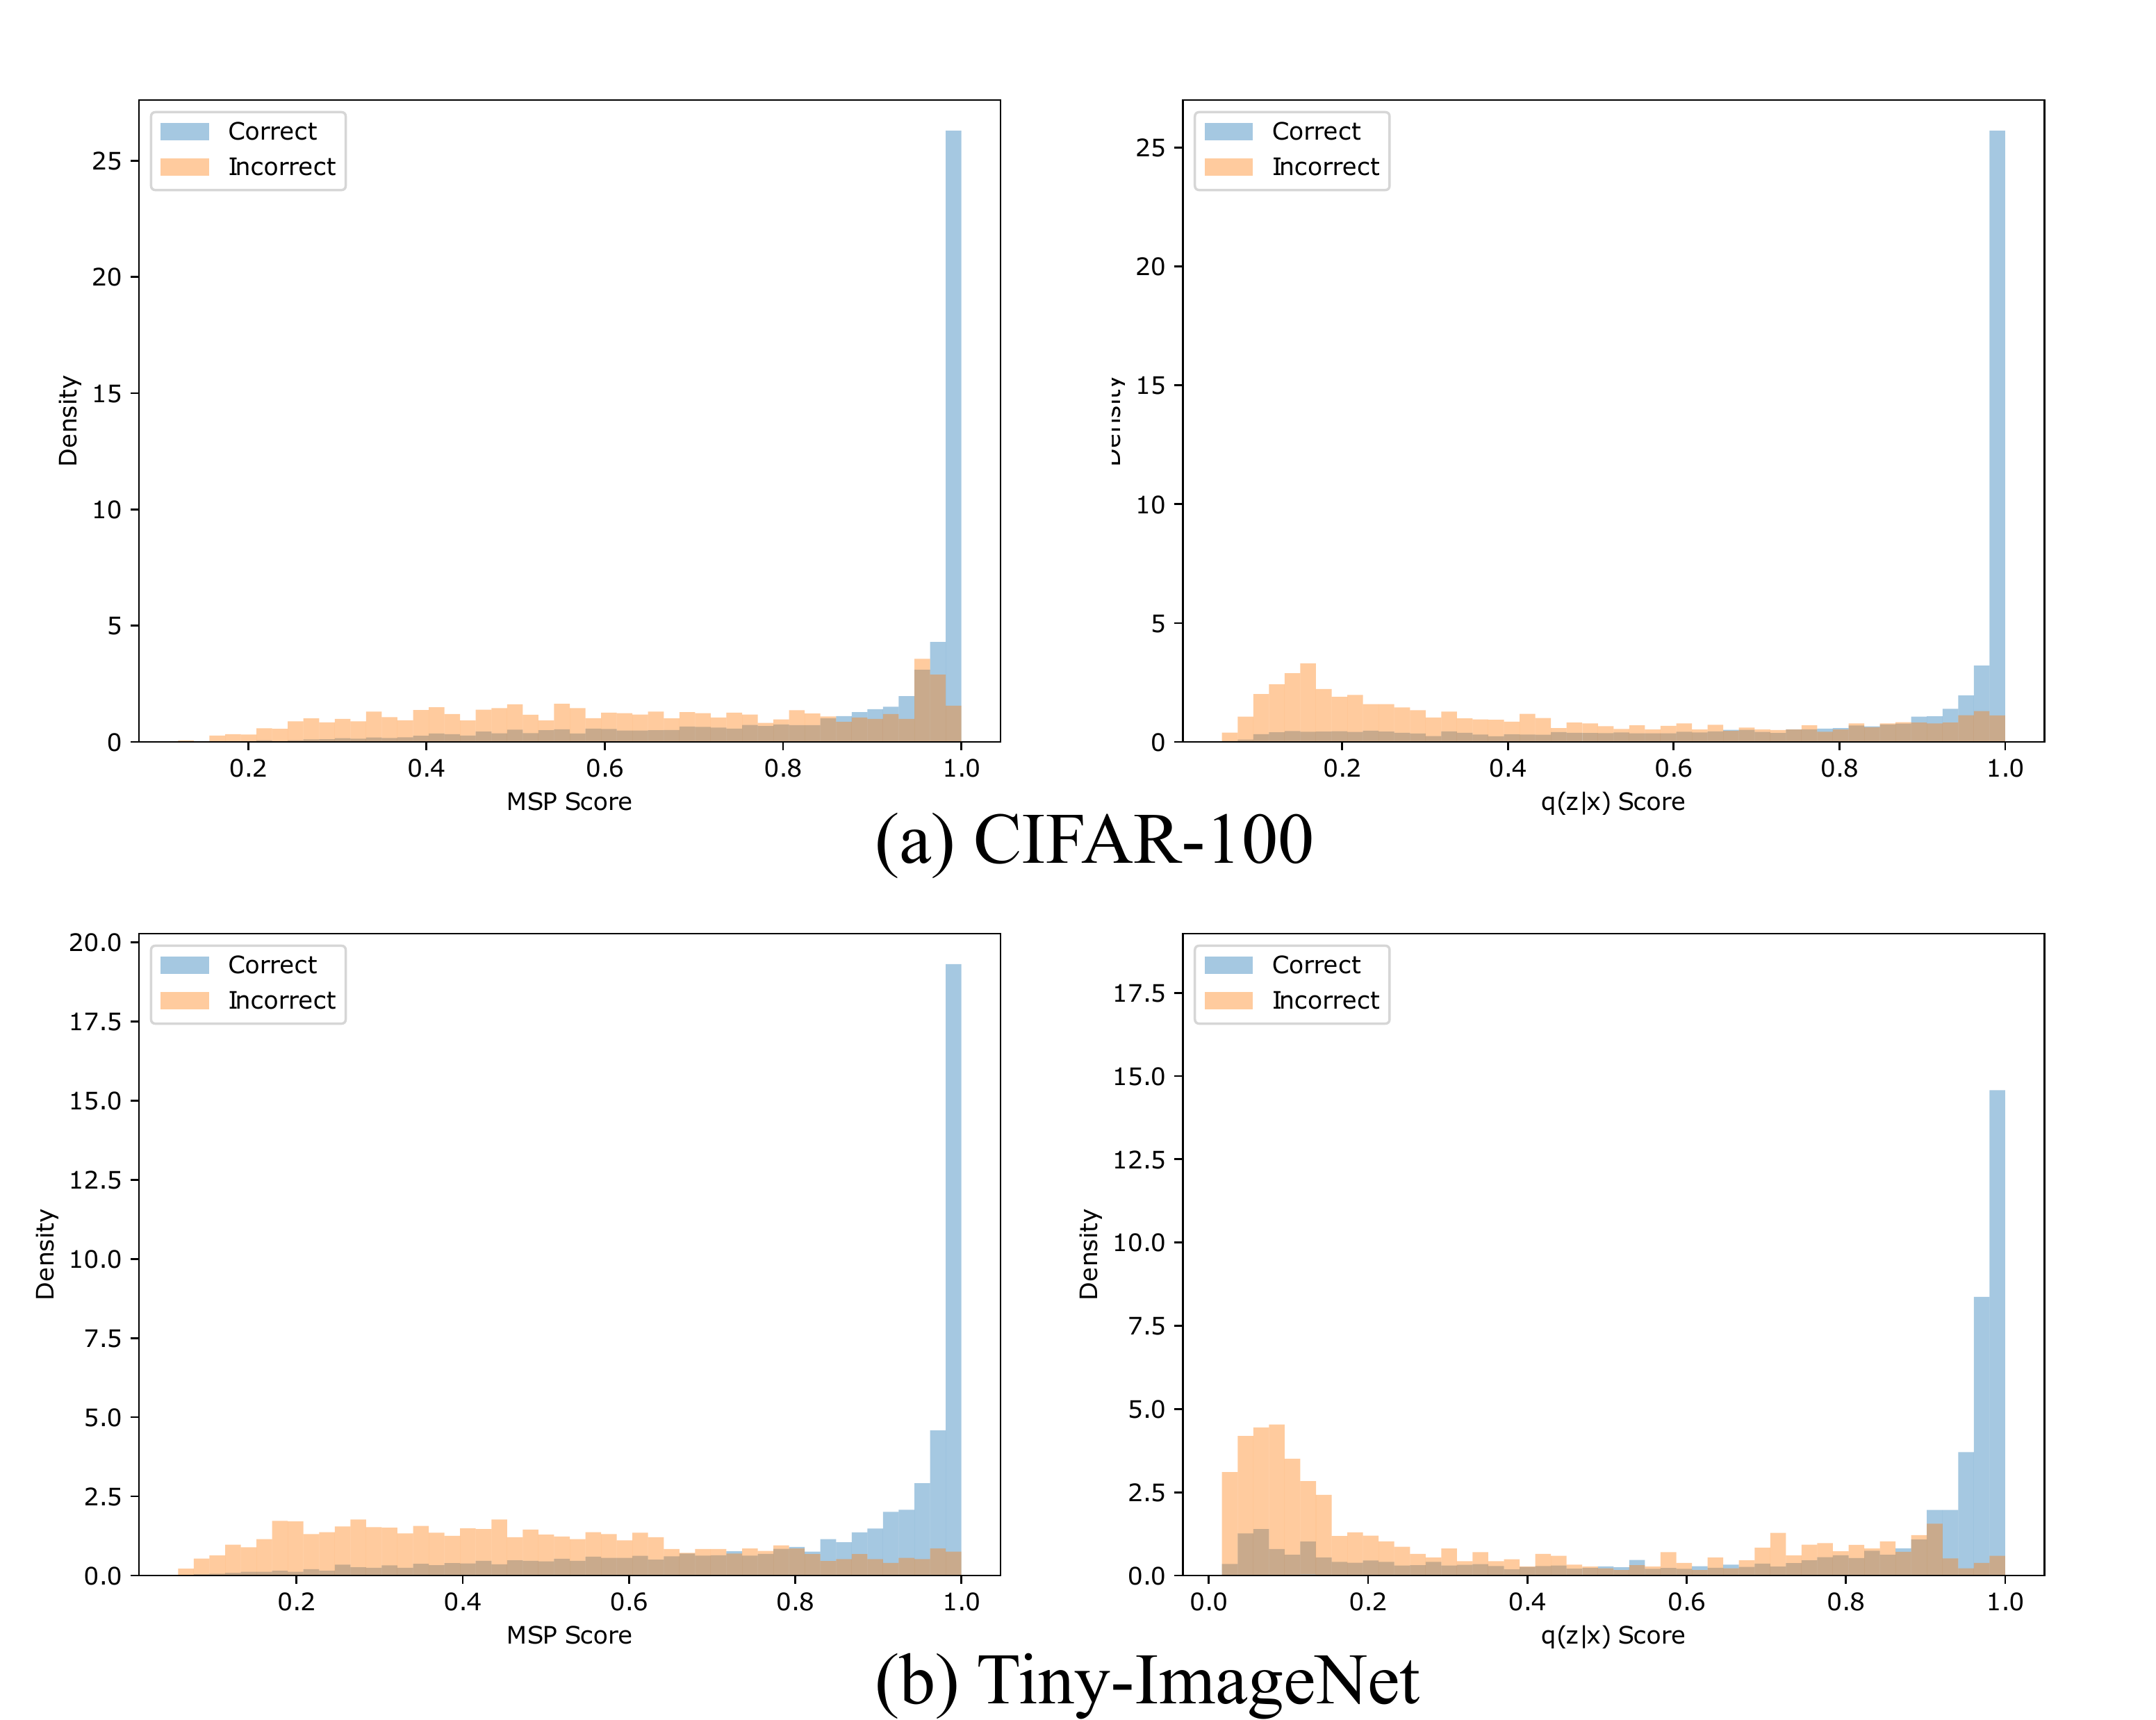}
	\caption{Histogram of MSP and AppealNet on CIFAR-100 and Tiny-ImageNet.}
	\label{fig:two-conf}
\end{figure}

\subsection{Black-Box Approximation}
\label{appendix:blackbox}
In Section~\ref{subsec:bl}, we show partial results of AppealNet under black-box settings. In this subsection, we show experimental results on CIFAR-100 and Tiny-ImageNet.  
Here, the little network is MobileNet and the baseline solution is MSP. The results of other settings are similar. 
The accuracy requirements are the same as previous ones: we evaluate the appealing rate (AR) of models under accuracy degradation AD $\in$ \{0.5\%, 1.0\%, 2.0\%, 5.0\%\}. %Note that the accuracy of AppealNet on GTSRB is high so that it is in-adequate
The results in the right part of Table 2 show the advantage of AppealNet over the baseline method. The relative improvement of AppealNet on CIFAR-100 and Tiny-ImageNet are up to 1.26x and 1.18x, respectively.

\begin{table*}[]
	\resizebox{\linewidth}{!}{
		\begin{tabular}{ccc|ccccccccc}
			\hline
			Dataset                        & \begin{tabular}[c]{@{}c@{}}Original\\ Accuracy\\ (\%)\end{tabular} & \begin{tabular}[c]{@{}c@{}}AppealNet\\ Accuracy\\ (\%)\end{tabular} & Method    & \begin{tabular}[c]{@{}c@{}}AR\\ at 0.5\%AD\\ (\%)\end{tabular} & \begin{tabular}[c]{@{}c@{}}Improvement\\ at 0.5\% AD\end{tabular} & \begin{tabular}[c]{@{}c@{}}AR\\ at 1.0\% AD\end{tabular} & \begin{tabular}[c]{@{}c@{}}Improvement\\ at 1.0\% AD\end{tabular} & \begin{tabular}[c]{@{}c@{}}AR\\ at 2.0\% AD\end{tabular} & \begin{tabular}[c]{@{}c@{}}Improvement\\ at 2.0\% AD\end{tabular} & \begin{tabular}[c]{@{}c@{}}AR\\ at 5.0\% AD\end{tabular} & \begin{tabular}[c]{@{}c@{}}Improvement\\ at 5.0\% AD\end{tabular} \\ \hline
			\multirow{2}{*}{CIFAR-100}     & \multirow{2}{*}{72.91}                                             & \multirow{2}{*}{72.57}                                              & MSP       & 69.70                                                          & 1.06x                                                             & 62.86                                                    & 1.17x                                                             & 53.85                                                    & 1.26x                                                             & 40.94                                                    & 1.20x                                                             \\
										   &                                                                    &                                                                     & AppealNet & 65.78                                                          & $\backslash$                                                      & 56.29                                                    & $\backslash$                                                      & 42.70                                                    & $\backslash$                                                      & 34.23                                                    & $\backslash$                                                      \\ \hline
			\multirow{2}{*}{Tiny-ImageNet} & \multirow{2}{*}{73.15}                                             & \multirow{2}{*}{73.11}                                              & MSP       & 70.15                                                          & 1.16x                                                             & 62.84                                                    & 1.18x                                                             & 52.08                                                    & 1.18x                                                             & 39.23                                                    & 1.16x                                                             \\
										   &                                                                    &                                                                     & AppealNet & 60.63                                                          & $\backslash$                                                      & 53.03                                                    & $\backslash$                                                      & 44.38                                                    & $\backslash$                                                      & 33.79                                                    & $\backslash$                                                      \\ \hline
			\end{tabular}}
	\caption{Appealing rate of black-box approximation under different accuracy requirements on CIFAR-100 and Tiny-ImageNet.}
	\label{tab:append-bl}
\end{table*}

{\small
\begin{table*}[]
	\centering
	\begin{tabular}{cccc|cccc}
		\hline
		\begin{tabular}[c]{@{}c@{}}Original\\ RMSE\\ (Pixels)\end{tabular} & \begin{tabular}[c]{@{}c@{}}Original\\ Acc.\\ (\%)\end{tabular} & \begin{tabular}[c]{@{}c@{}}AppealNet\\ RMSE\\ (Pixels)\end{tabular} & \begin{tabular}[c]{@{}c@{}}AppealNet\\ Acc.\\ (\%)\end{tabular} & \begin{tabular}[c]{@{}c@{}}SR\\ at 0.5\%AD\\ (\%)\end{tabular} & \begin{tabular}[c]{@{}c@{}}SR\\ at 1.0\%AD\\ (\%)\end{tabular} & \begin{tabular}[c]{@{}c@{}}SR\\ at 2.0\%AD\\ (\%)\end{tabular} & \begin{tabular}[c]{@{}c@{}}SR\\ at 5.0\%AD\\ (\%)\end{tabular} \\ \hline
		2.35                                                               & 95.24                                                          & 2.47                                                                & 94.93                                                           & 66.79                                                          & 75.50                                                          & 88.79                                                        & 99.93                                                        \\ \hline
		\end{tabular}
\caption{Skipping rate under different accuracy requirements on facial keypoints detection.}
\label{tab:reg}
\end{table*}
}

\section{AppealNet on Regression Task: Facial Keypoints Detection}
\label{appendix:reg}
The optimization objective derived in Section~\ref{subsec:or} is also applicable to common regression tasks by replacing the loss function from cross-entropy to $L2/L1$ or other forms of loss. Thus, in this section, we take \textit{facial keypoints detection} as a case study to illustrate the potential of AppealNet on regression tasks.
The objective of facial keypoints detection is to predict keypoint coordinates on face images. 

\textbf{Dataset:} 
We use the data provided by \textit{Kaggle's facial keypoints detection challenge}, wherein 15 keypoints are labeled on face images. There are 7,094 labeled images. We split the data into two parts: 80\% for training and 20\% for testing. 
Figure~\ref{fig:face-sample} shows four random samples and their keypoint labels (red dots) in the dataset.

\textbf{Neural Network:}
The neural network design for AppealNet on regression tasks is similar to the one for classification tasks. We adopt the baseline model for this task and insert the predictor head to construct AppealNet.
To be more specific, the approximator is a convolutional neural network with 3 convolutional layers followed by 2 fully-connected layers. The output of the approximator is a 30-dim vector specifying 15 keypoints' coordinates.
An auxiliary fully-connected layer is inserted into network as predictor head. Since we evaluate AppealNet under black-box setting here, the big network is considered as an oracle, which always yields ground-truth labels.

\begin{figure}[t]
	\centering
	\includegraphics[width=\linewidth]{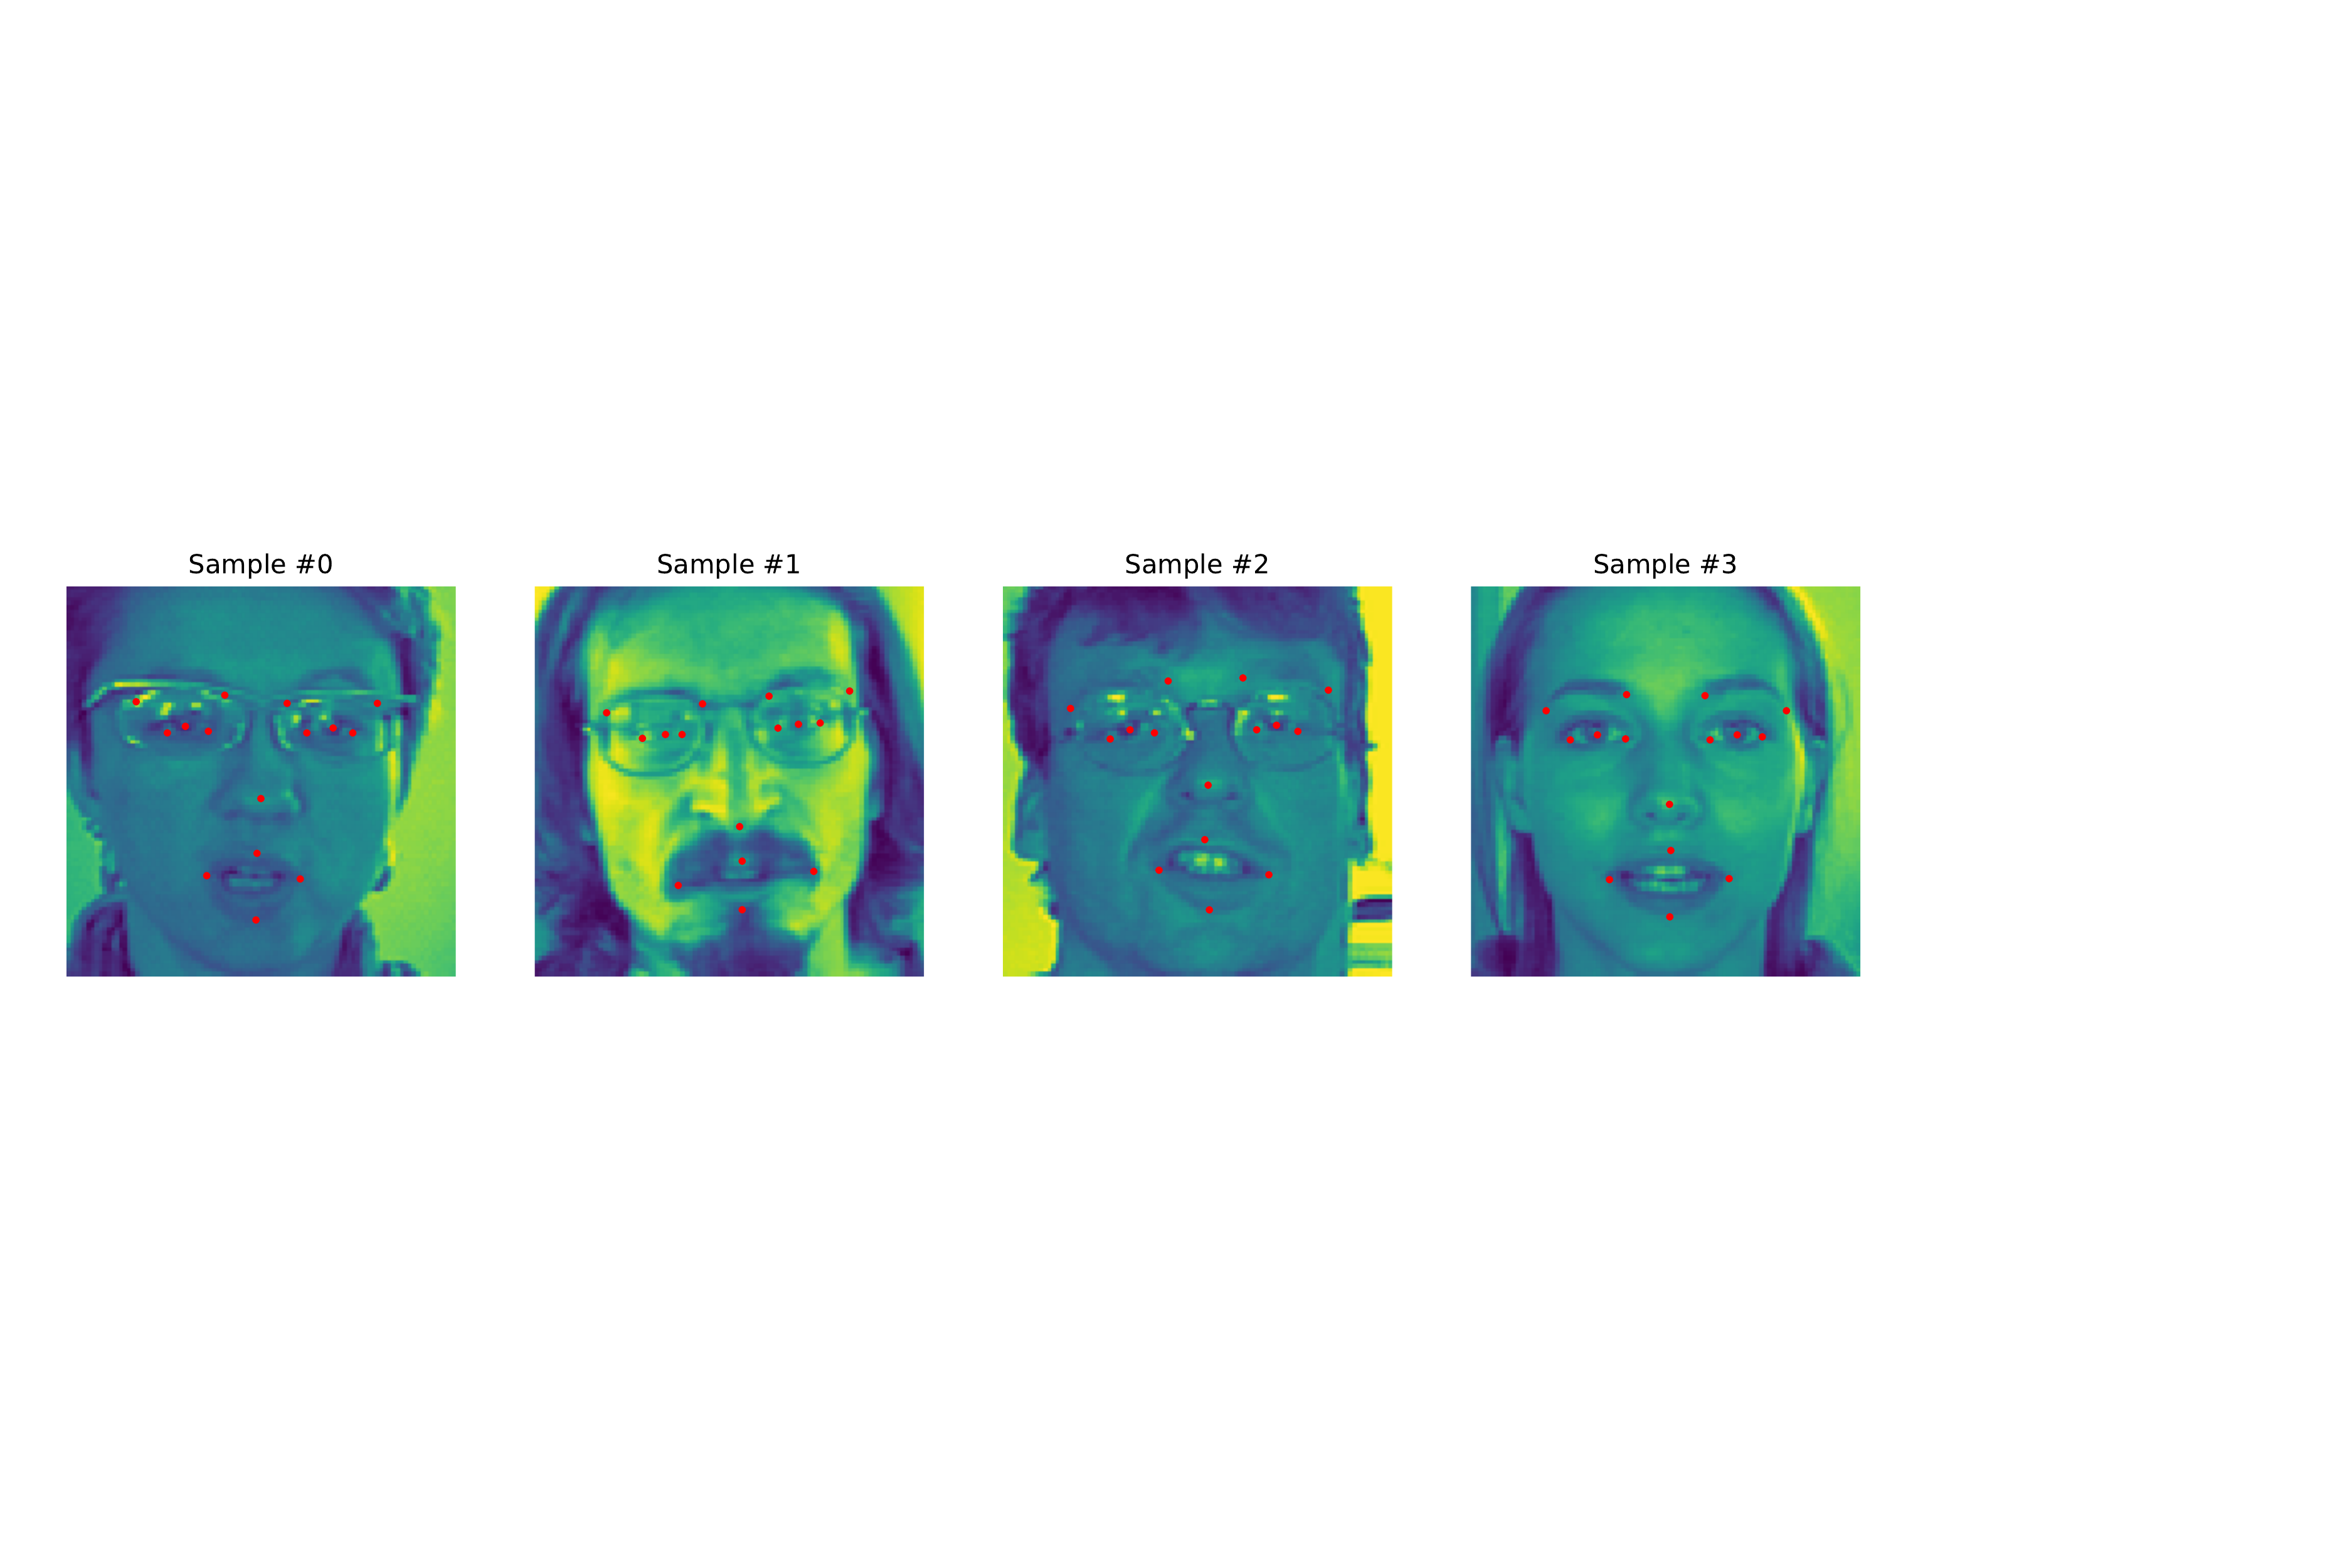}
	\caption{Samples from Kaggle's facial keypoints detection.}
	\label{fig:face-sample}
\end{figure}

\textbf{Evaluation Metrics:} 
The main difference between regression tasks and classification tasks under AppealNet setting is the definition of \textit{accuracy} (Eq.~\eqref{eq:overall-acc}), as the outputs of networks are continues values instead of discrete categories. We adopt a straightforward yet reasonable definition of an \textit{accurate inference}: the error of predicted labels $f(\mathbf{x})$ with respect to the ground-truth label $y$ is within an acceptable range, and this range is application-dependent. Such definition is consistent with conventional metrics applied in regression-based computer vision tasks, for example \textit{Accuracy @.50IoU} (Accuracy when correct inference is defined as \textit{Intersection of Union} of predicted bounding box and ground-truth is larger than 50\%) for object detection.
As for facial keypoints detection, concerning the original image sizes (96x96) and the precision of keypoints labeling, we safely assume that if the Euclidean distance/RMSE (\textit{i.e.,} root square of $L2$ distance) between the predicted keypoint coordinates and the ground-truth is 
\textbf{less than 4 pixels}, the inference is accurate and hence can be accepted by the little network. 

Based on the above modification on \textit{accurate inference} for regression task, we evaluate AppealNet using the skipping rate (SR) and the accuracy drop (AD) defined in Section~\ref{sec:exp}.

\textbf{Effectiveness of AppealNet:} 
We investigate the effectiveness of AppealNet under black-box settings, where the degradation of the system accuracy comes from the misclassification of the little network. 
First, both RMSE and Accuracy of AppealNet are close to those of the original network (See first 4 columns in Table~\ref{tab:reg}), which shows that AppealNet has little impact on regression accuracy. 
Second, we report the skipping rate under accuracy degradation AD $\in$ \{0.5\%, 1.0\%, 2.0\%, 5.0\%\}. A higher skipping rate means more computations on the approximator, thereby saving more energy. 
The results in the right part of Table~\ref{tab:reg} show that AppealNet can guarantee highly-accurate inference while keeping a large portion of inputs being processed by the little network. For example, we can keep 75.50\% of inputs on the approximator for computation when system accuracy is above 99.0\% (See 6$^{th}$ column). Note that, no baseline solutions is given here, because all previous solutions are only applicable to classification tasks and we have no access to "confidence" information from the original networks to adapt them for regression tasks. %From this perspective, AppealNet enables neural networks for regression tasks to estimate confidence on specific inputs. Such capability is highly needed for some security-sensitive applications. 

%We will extend AppealNet to more sophisticated AI tasks, either classification or regression, in our future work.
